# Supplementary material for: Interplay between organic cations and inorganic framework and incommensurability in hybrid lead-halide perovskite CH3NH3PbBr3
Source: arXiv:1705.10691 ancillary file (2017-08-29)
Supplement: Supplementary file 1 [file SI.pdf]

# Supplementary Information: Interplay between organic cations and inorganic framework and incommensurability in hybrid lead-halide perovskite $\text{CH}_3\text{NH}_3\text{PbBr}_3$

Yinsheng Guo,<sup>1</sup> Omer Yaffe,<sup>2</sup> Daniel W. Paley,<sup>1,3</sup> Alexander N. Beecher,<sup>1</sup> Trevor D. Hull,<sup>1</sup> Guilherme Szpak,<sup>4,1</sup> Jonathan S. Owen,<sup>1</sup> Louis E. Brus,<sup>1</sup> and Marcos A. Pimenta<sup>4,1,\*</sup>

<sup>1</sup>*Department of Chemistry, Columbia University, New York, NY 10027, USA*

<sup>2</sup>*Department of Materials and Interfaces, Weizmann Institute of Science, Rehovot, 76100, Israel*

<sup>3</sup>*Columbia Nano Initiative, Columbia University, New York NY 10027*

<sup>4</sup>*Departamento de Física, Universidade Federal de Minas Gerais, 30123-970 Belo Horizonte, Brazil*

(Dated: August 22, 2017)

## Experimental methods

**Single crystal synthesis** The synthesis of  $\text{CH}_3\text{NH}_3\text{PbBr}_3$  single crystals has been previously reported.[1] Briefly,  $\text{CH}_3\text{NH}_3\text{Br}$  was prepared from aqueous  $\text{CH}_3\text{NH}_2$  solution (40% w/w Alfa Aesar) and  $\text{HBr}$  acid (48% Acros).  $\text{PbBr}_2$  (98% Sigma-Aldrich) and  $\text{CH}_3\text{NH}_3\text{Br}$  was dissolved in  $\text{N,N}$ -dimethylformamide to prepare 1M solution of 1:1 ratio.  $\text{CH}_3\text{NH}_3\text{PbBr}_3$  crystals were grown by diffusion of isopropyl alcohol vapor into the prepared solution. For  $\text{CsPbBr}_3$ , small, orange single crystals were grown by diffusion of  $n$ -propyl alcohol vapor into a 30 mM solution of 1:1  $\text{PbBr}_2$  (98%, Sigma-Aldrich) and  $\text{CsBr}$  (99% metal basis, Alfa Aesar) in  $\text{N,N}$ -dimethylformamide.

**Single crystal X-ray diffraction** All single-crystal diffraction data was collected on an Agilent SuperNova diffractometer using mirror-monochromated or  $\text{Mo K}\alpha$  radiation. Data collection, integration, scaling (ABSPACK) and absorption correction (face-indexed Gaussian integration[2]) were performed in CrysAlisPro. Structure solution was performed using ShelXT.[3] Subsequent refinement was performed by full-matrix least-squares on  $F^2$  in ShelXL.[4] Olex2[5] was used for viewing and to prepare CIF files.

**Low-frequency Raman spectroscopy** The low-frequency Raman scattering was measured on a home-built confocal micro Raman setup. The 633nm line of a Helium-Neon laser was used as the excitation. Sub-bandgap, pre-resonance excitation provides signal enhancement while minimizes possible degradation issues as noted in literature for  $\text{CH}_3\text{NH}_3\text{PbI}_3$ . [6, 7] A Nikon 40x long working distance objective ( $\text{NA}=0.6$ ) was used to both focus the laser and collect scattered light. A 90/10 volume holographic beam splitter was used to couple the excitation on the sample and transmit frequency-shifted signal to detection. Two volume holographic notch filters, each with  $\text{OD}>4$ , were used to attenuate the Rayleigh line. The Raman scattered light was dispersed by a single stage spectrograph with a 1800 grooves/mm diffraction grating, and collected by a liquid nitrogen cooled CCD. The samples were held in an optical cryostat, with an operation pressure level of  $1 \times 10^{-5}$  torr. The sample temperature was controlled by liquid nitrogen flow and local heater on the sample stage. Due to its first order nature, the phase transition temperature of  $\text{CH}_3\text{NH}_3\text{PbBr}_3$  exhibit a thermal hysteresis of about 10 K during the cooling-warming cycles, similar to previous report.[8] Samples were stable during the experiments with reproducible spectral features and evolution from multiple cooling-warming cycles. No spectral feature or morphology change from degradation was observed at any time.

## Halide mode at $\approx 320\text{cm}^{-1}$

The phonon mode at  $\approx 320\text{cm}^{-1}$  exists in both  $\text{CH}_3\text{NH}_3\text{PbBr}_3$  and  $\text{CsPbBr}_3$  as shown in figure S1. Several previous studies assign this mode to the torsional vibration of  $\text{CH}_3\text{NH}_3^+$ . [7, 9] Yet, the comparison between  $\text{CH}_3\text{NH}_3\text{PbBr}_3$  and  $\text{CsPbBr}_3$  indicates that the internal motion of the  $\text{CH}_3\text{NH}_3^+$  cation is not a necessary component for this mode. Corresponding mode has been observed in chloride perovskites with a frequency shift that agrees with simple estimate based on different halide masses of a harmonic oscillator. In addition, the drastic mass difference between A site cations of  $\text{CH}_3\text{NH}_3^+$  ( $M=32$ ) and  $\text{Cs}$  ( $M=132.9$ ) does not significantly affect the frequency of this mode, further suggesting the minimal role of A cations. All observations above indicate that this mode belongs predominantly to the perovskite octahedral framework, composed primarily of halide motion.

---

\* mpimenta@fisica.ufmg.br

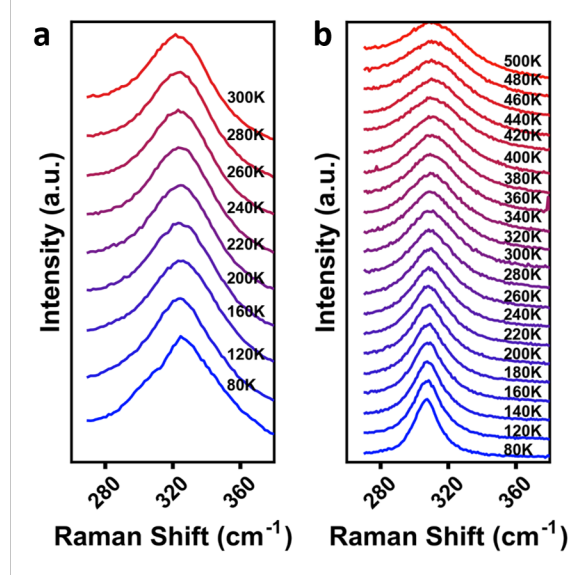

FIG. 1: Raman modes around  $320\text{cm}^{-1}$  in both (a)  $\text{CH}_3\text{NH}_3\text{PbBr}_3$  and (b)  $\text{CsPbBr}_3$

### Twinned basic structures

As the crystal transition below the tetragonal phase, a two-fold twinning develops and results in an additional split reflection. The strong twinning reflection hampers the full structural characterization of the incommensurate modulation. We solved and refined the twinned basic structure by omitting satellite reflections from the data set; this new structure is shown below.

*Transformation matrices* Since data for the three phases were collected successively, it was possible to use a common orientation matrix to reveal the geometric relationship between the phases. The tetragonal direct basis is transformed to the incommensurate phase by the matrix (rounded to omit changes in cell volume):

$$\begin{pmatrix} a \\ b \\ c \end{pmatrix}_{inc} = \begin{pmatrix} -1/2 & -1/2 & 1/2 \\ 1 & -1 & 0 \\ 1/2 & 1/2 & 1/2 \end{pmatrix} \begin{pmatrix} a \\ b \\ c \end{pmatrix}_{tI} \quad (1)$$

A second twin-related domain is given by twofold rotation around the 110 vector of the tetragonal cell. The incommensurate phase is transformed to the orthorhombic Pnma phase by the matrix:

$$\begin{pmatrix} a \\ b \\ c \end{pmatrix}_{oP} = \begin{pmatrix} -1/2 & 1/2 & 1/2 \\ 1 & 0 & 1 \\ -1/2 & -1/2 & 1/2 \end{pmatrix} \begin{pmatrix} a \\ b \\ c \end{pmatrix}_{inc} \quad (2)$$

Note that this transformation gives back the original axes with b and c exchanged. The second twin-related domain of the incommensurate phase is transformed by the same matrix. Furthermore, two additional twin domains can be resolved for the Pnma phase with occupancy  $<10\%$  each. These seem to derive from a 12% occupied minor twin component of the tetragonal phase, but it is unclear how the crystal "remembers" these domain boundaries, since the orientation of the tetragonal c axis is lost in the incommensurate phase. Perhaps domain boundaries are pinned to defects or strain in the crystal.

### Coexistence of the incommensurate and commensurate phase at 148K

Interestingly, reflections of the incommensurate Imma satellite reflections and the commensurate orthorhombic Pnma lattice reflections were observed to coexist at 148K, as shown in figure 2. This result can be explained by the coexistence of the two phases due to the first-order nature of the phase transition, but can also be the

signature of the multi-solitons regime of an incommensurate modulation, where commensurate domains separated by discommensurations appear in the crystalline structure.

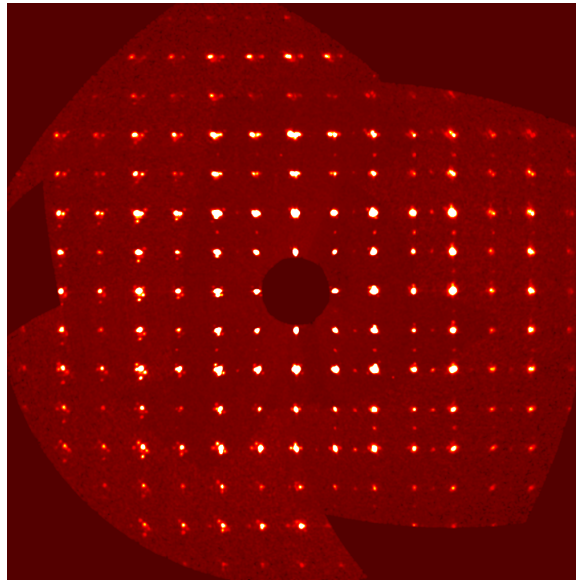

FIG. 2: A synthetic precession frame showing coexisting modulated and Pnma phases. Satellite reflections from the incommensurate modulation are observed, for instance, on the left side of the image. The additional reflections of the orthorhombic Pnma lattice can be seen at halfway between main reflections, for instance, on the right side of the image.

- 
- [1] O. Yaffe, Y. Guo, L. Z. Tan, D. A. Egger, T. Hull, C. C. Stoumpos, F. Zheng, T. F. Heinz, L. Kronik, M. G. Kanatzidis, J. S. Owen, A. M. Rappe, M. A. Pimenta, and L. E. Brus, *Phys. Rev. Lett.* **118**, 136001 (2017).
  - [2] E. Blanc, D. Schwarzenbach, and H. D. Flack, *Journal of Applied Crystallography* **24**, 1035 (1991).
  - [3] G. M. Sheldrick, *Acta Crystallographica Section A* **71**, 3 (2015).
  - [4] G. M. Sheldrick, *Acta Crystallographica Section A* **64**, 112 (2008).
  - [5] O. V. Dolomanov, L. J. Bourhis, R. J. Gildea, J. A. K. Howard, and H. Puschmann, *Journal of Applied Crystallography* **42**, 339 (2009).
  - [6] M. Ledinský, P. Löper, B. Niesen, J. Holovský, S.-J. Moon, J.-H. Yum, S. De Wolf, A. Fejfar, and C. Ballif, *J. Phys. Chem. Lett.* **6**, 401 (2015).
  - [7] A. M. A. Leguy, A. R. Goni, J. M. Frost, J. Skelton, F. Brivio, X. Rodriguez-Martinez, O. J. Weber, A. Pallipurath, M. I. Alonso, M. Campoy-Quiles, M. T. Weller, J. Nelson, A. Walsh, and P. R. F. Barnes, *Phys. Chem. Chem. Phys.* **18**, 27051 (2016).
  - [8] K. Futterer, R. L. Withers, T. R. Welberry, and W. Depmeier, *Journal of Physics: Condensed Matter* **7**, 4983 (1995).
  - [9] A. Maalej, Y. Abid, A. Kallel, A. Daoud, A. Lautié, and F. Romain, *Solid State Commun.* **103**, 279 (1997).
